# Supplementary material for: Homogeneous ice nucleation in an ab initio machine learning model of water
Source: arXiv:2203.01376 ancillary file (2022-08-24)
Supplement: Supplementary file 1 [file supplementary_information.pdf]

PNAS
www.pnas.org

# Supplementary Information for

## Homogeneous ice nucleation in an ab initio machine learning model of water

**Pablo M. Piaggi, Jack Weis, Athanassios Z. Panagiotopoulos, Pablo G. Debenedetti and Roberto Car**

**Pablo M. Piaggi - E-mail: ppiaggi@princeton.edu**
**Roberto Car - E-mail: rcar@princeton.edu**

### This PDF file includes:

Supplementary text
Figs. S1 to S12
Tables S1 to S2
SI References

## Supporting Information Text

### 1. Choice of system size for seeding simulations

We chose the number of water molecules in the seeding simulation based on the recommendation of Espinosa et al. (1). They suggest to employ approximately twenty times more water molecules in the simulation box than the water molecules in the simulated cluster. We analyzed the rationale of this criterion in the following way. We consider a spherical ice cluster of $N_c$ molecules and radius $r$, in a cubic box with $N$ liquid water molecules. We use the symbol $a$ for the distance from the surface of the spherical cluster to the edge of the box (see scheme in Fig. S1). Assuming that each phase has its bulk density, the ratio

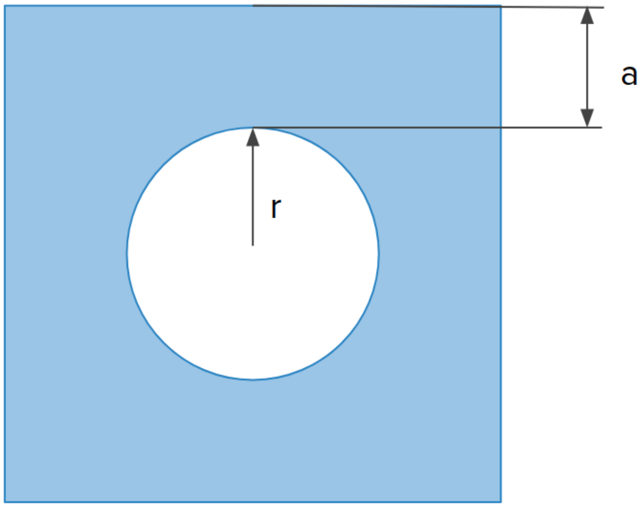


**Fig. S1. Scheme for choice of system size in the seeding simulations.** An ice cluster of radius $r$ is embedded in a cubic box. We use the symbol $a$ for the distance from the surface of the spherical cluster to the edge of the box.

between $N$ and $N_c$ is,

$$\frac{N}{N_c} = 1 + \left( \frac{6(a+r)^3}{\pi r^3} - 1 \right) \frac{\rho_{\text{water}}}{\rho_{\text{ice}}}, \qquad [1]$$

where $\rho_{\text{water}}$ and $\rho_{\text{ice}}$ are the densities of water and ice, respectively. A possible choice for $a$ is $a = r$ that represents a spacing $2r$ between ice clusters in neighboring periodic images. This is a very conservative choice considering that we expect no long-range interactions (the electrostatic interaction will be screened in water and ice) and that the correlation length in the liquid is around 1 nm. This choice leads to,

$$\frac{N}{N_c} = 1 + \left( \frac{48}{\pi} - 1 \right) \frac{\rho_{\text{water}}}{\rho_{\text{ice}}} \approx 16, \qquad [2]$$

in good agreement with the criterion of Espinosa et al.

The choice of system size for our seeding simulations and the $N/N_c$ ratio are summarized in Table S1.

| $N_c$ | $N$ | $N/N_c$ |
|---|---|---|
| 190 | 3 934 | ∼21 |
| 688 | 11 872 | ∼17 |
| 4 676 | 99 404 | ∼21 |

**Table S1. Choice of system size in the seeding simulations.** $N_c$ **is the number of molecules in the ice cluster and** $N$ **is the total number of water molecules in the cubic simulation box.**

### 2. Results of the seeding simulations

In order to determine the temperature $T^*$ for which a given cluster is critical we performed molecular dynamics simulations at different temperatures. The results of these simulations are shown in Fig. S2.

From these simulations we identified the temperatures shown in Table S2. In Figures where quantities are plotted against supercooling we have added an extra 1 K to the error $\Delta T^*$ to take into account that the melting temperature is not know precisely.

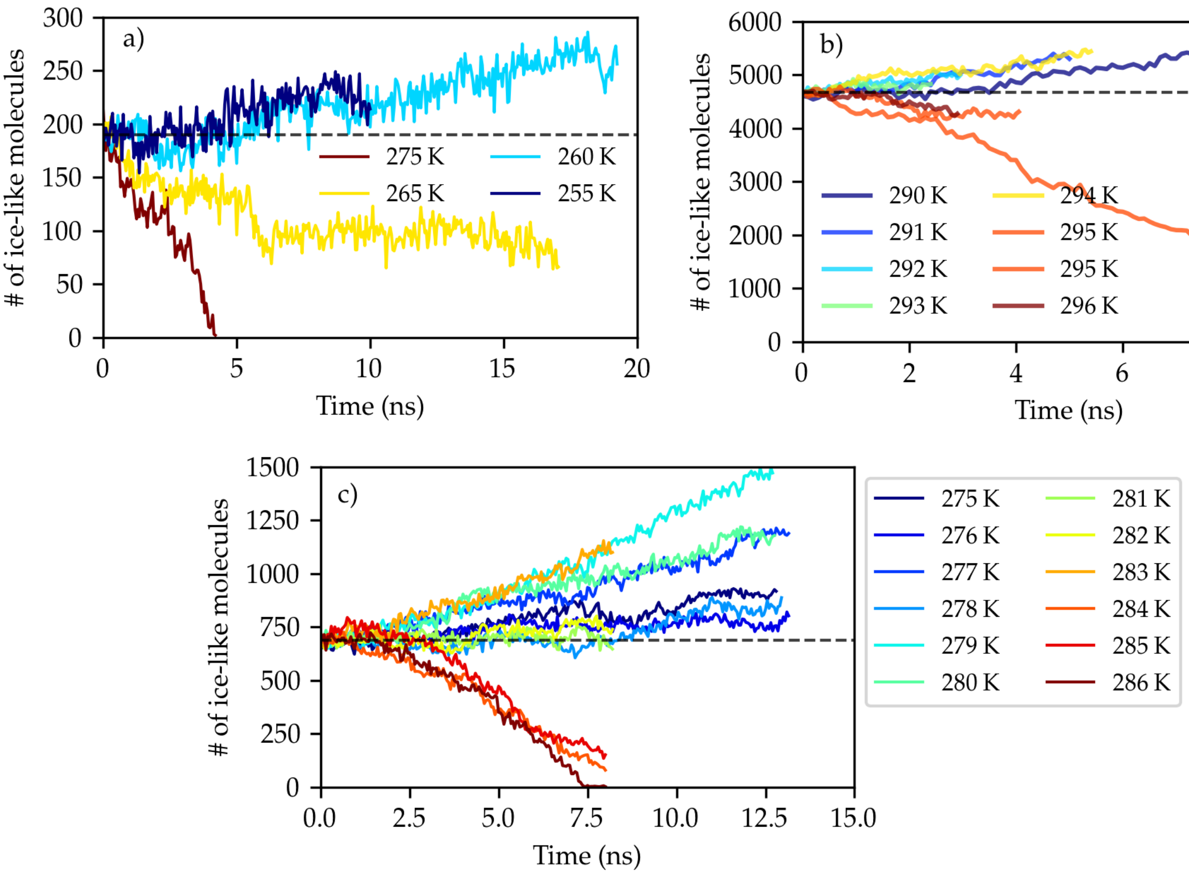


**Fig. S2. Results of the seeding simulations.** Number of ice-like molecules as a function of simulation time for the three systems sizes studied in this work. The total number of molecules in the simulation boxes are 3 934, 99 404, and 11 872 for subplots a), b), and c), respectively.

| $N^*$ | $T^*$ | $\Delta T^*$ |
|---|---|---|
| 190 | 267.5 | 3.5 |
| 688 | 282 | 2 |
| 4 676 | 294.5 | 1.5 |

**Table S2. Temperatures $T^*$ at which a cluster of size $N^*$ is critical for the three clusters studied in this work. Error $\Delta T^*$ is also shown.**

## 3. Relaxation times of liquid water

We computed the correlation times of the potential energy in liquid water at different temperatures. The results are shown in Fig. S3. The correlation times increase significantly below 280 K and are longer than ∼1 ns below 260 K. The smallest cluster

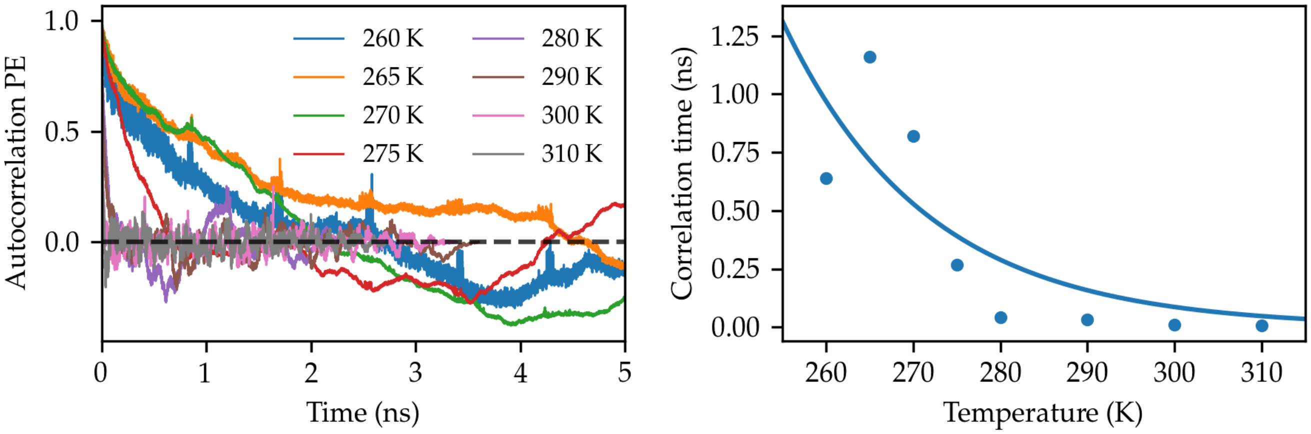


**Fig. S3. Relaxation times in SCAN-ML liquid water.** Left) Autocorrelation function of the potential energy. Right) Correlation times $\tau$ calculated based on a fit of the autocorrelation functions to $e^{-t/\tau}$. The solid line is based on a fit to the data using an exponential functional form.

used in the seeding simulations was equilibrated at 240 K and production runs were performed at temperatures between 255 and 275 K. Due to the long relaxation times, in these simulations the cluster can grow or shrink during the progression towards equilibrium.

## 4. Errors in seeding simulations

We calculated the errors in our estimate for the nucleation rate by error propagation starting from Eq. (1) of the main text. The error $\delta_J$ in the nucleation rate $J$ is:

$$\delta_J = J\left(\left(\frac{1}{\rho_l}\right)^2 \delta_{\rho_l}^2 + \left(\frac{1}{f^+}\right)^2 \delta_{f^+}^2 + \left(\frac{1}{2|\Delta\mu|} - \frac{N^*}{2k_BT}\right)^2 \delta_{|\Delta\mu|}^2 + \left(-\frac{1}{2T} + \frac{N^*|\Delta\mu|}{2k_BT^2} + \frac{|\Delta\mu|'}{2|\Delta\mu|} - \frac{N^*|\Delta\mu|'}{2k_BT} + \frac{\rho_l'}{\rho_l} + \frac{f^{+\prime}}{f^+}\right)^2 \delta_T^2\right)^{1/2},$$

where $\delta_x$ is the error is some property $x$, $x'$ denotes the first derivative of $x$, and the rest of the symbols have the same meaning as in Eq. (1). Since $J$ is typically plotted in log scale we calculated the error:

$$\delta_{\log_{10}(J)} = \log_{10}(e)\frac{\delta_J}{J} \qquad [3]$$

that is shown with error bars in Fig. 2.

We also calculated the error $\delta_\gamma$ in the interfacial free energy $\gamma$ starting from Eq. (3) of the main text. The error is:

$$\delta_\gamma = \gamma\left(\left(\frac{\delta_{|\Delta\mu|}}{|\Delta\mu|}\right)^2 + \left(\frac{2\delta_{\rho_{\text{ice}}}}{3\rho_{\text{ice}}}\right)^2 + \left(\frac{|\Delta\mu|'}{|\Delta\mu|} + \frac{2\rho_{\text{ice}}'}{3\rho_{\text{ice}}}\right)^2 \delta_T^2\right)^{1/2}. \qquad [4]$$

In the error formulas we have included the explicit errors in the quantities in the equations for $J$ and $\gamma$, and also the implicit error due to the dependence of several quantities on the temperature.

## 5. Turnbull/Laird correlation

We analyzed the correlation between the interfacial free energy and the melting temperature in different models(2, 3). Results are shown in Fig. S4. The interfacial free energy of mW clearly deviates from the trend of the other models. This behavior is likely a consequence of different physics resulting from the lack of protons in the model.

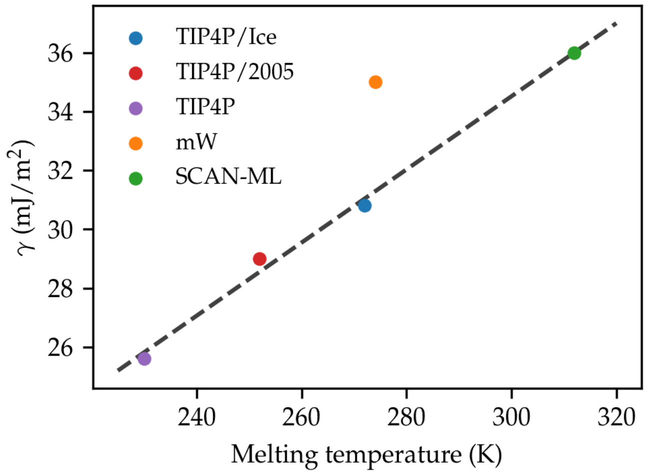


**Fig. S4. Correlation between the interfacial free energy and the melting temperature in different models.** Results for the TIP4P family and mW from Espinosa et al. (4).

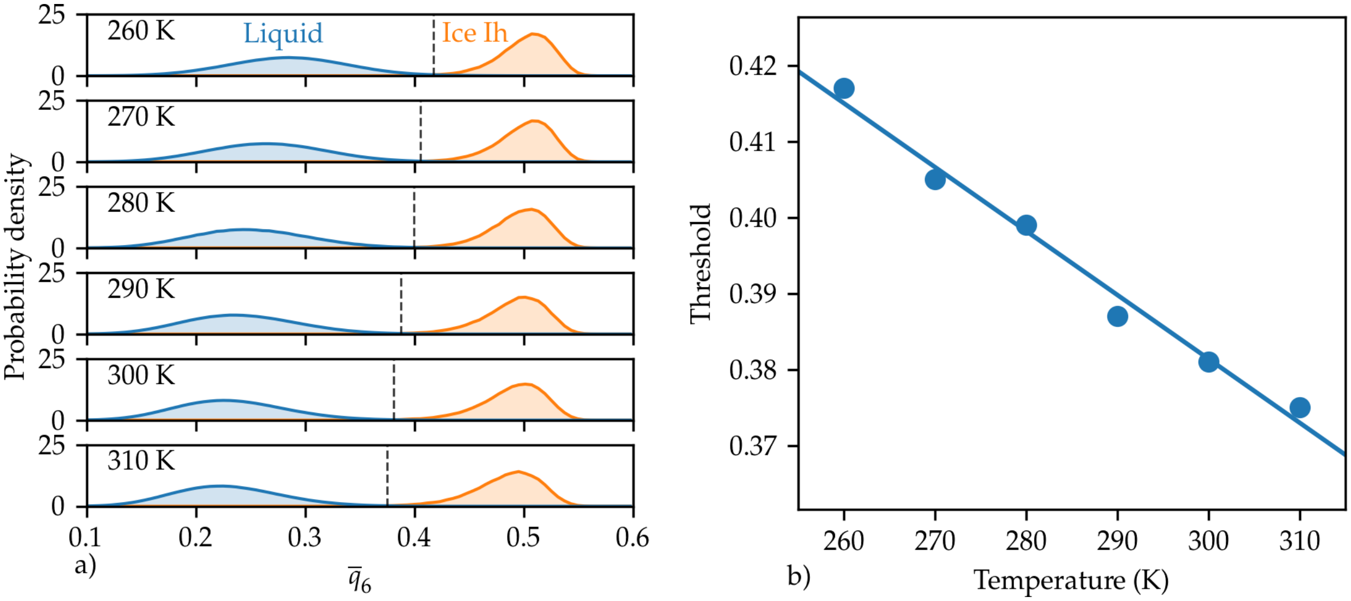


**Fig. S5. Criterion to differentiate liquid-like and ice-like environments.** a) Probability distributions of the order parameter $\bar{Q}_6$ in liquid water and ice Ih. The threshold value of $\bar{Q}_6$ used to distinguish liquid water and ice Ih is shown with a vertical dashed line. b) Threshold as a function of temperature and a linear fit to the data.

## 6. Criterion to differentiate liquid-like and ice-like environments

We employed the local Steinhardt parameter $\bar{Q}_6$ proposed by Lechner and Dellago(5) to differentiate liquid-like and ice Ih-like environments. The distributions of $\bar{Q}_6$ for the liquid and ice Ih at 1 bar and different temperatures are shown in Fig. S5a. There is good separation between the liquid and ice Ih distributions although the dividing line between the two phases shifts to the right as a function of temperature. We defined the threshold value of $\bar{Q}_6$ to classify environments based on the following criterion. We use the symbols $p_l(\bar{Q}_6)$ and $p_i(\bar{Q}_6)$ to denote the probability distributions of $\bar{Q}_6$ in the liquid and ice Ih, respectively. The threshold $\bar{Q}_6{}^*$ satisfies $p_l(\bar{Q}_6{}^*) = p_i(\bar{Q}_6{}^*)$ and $p_l(\bar{Q}_6{}^*) > \epsilon, p_i(\bar{Q}_6{}^*) > \epsilon$ with $\epsilon \approx 0$. The latter conditions avoid the trivial solution $p_l(\bar{Q}_6{}^*) = p_i(\bar{Q}_6{}^*) \approx 0$ that might be satisfied to the left of the liquid distribution or to the right of the ice Ih distribution. This criterion is equivalent to requiring that an atomic environment characterized by $\bar{Q}_6{}^*$ has equal probabilities of being classified as liquid or ice Ih.

The threshold as a function of temperature is shown in Fig. S5b and shows a strong linear correlation. We employed this linear fit to determine the appropriate threshold at a given temperature.

We also considered the overlap $\Theta$ between $p_l(\bar{Q}_6)$ and $p_i(\bar{Q}_6)$ defined as,

$$\Theta(p_l, p_i) = \int d\bar{Q}_6 \min[p_l(\bar{Q}_6), p_i(\bar{Q}_6)], \quad [5]$$

where $\min[p_l(\bar{Q}_6), p_i(\bar{Q}_6)]$ is the minimum between $p_l$ and $p_i$ for a given $\bar{Q}_6$. $\Theta(p_l, p_i)$ as a function of temperature is shown in Fig. S6 and shows a sharp increase below 270 K, compatible with the location of the Widom line.

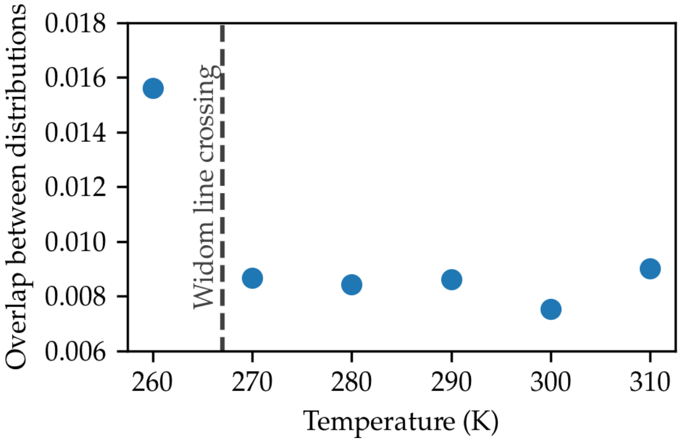


**Fig. S6. Overlap between the probability distributions of $\bar{Q}_6$ in liquid water and ice Ih.** The location of the Widom line at 1 bar is shown with a vertical dashed line.

## 7. Calculation of attachment rates

The calculated attachment rates are shown in Fig. S7 for the three cluster sizes considered in this work. The exponential fit used to calculate the nucleation rate as a function of temperature is also shown.

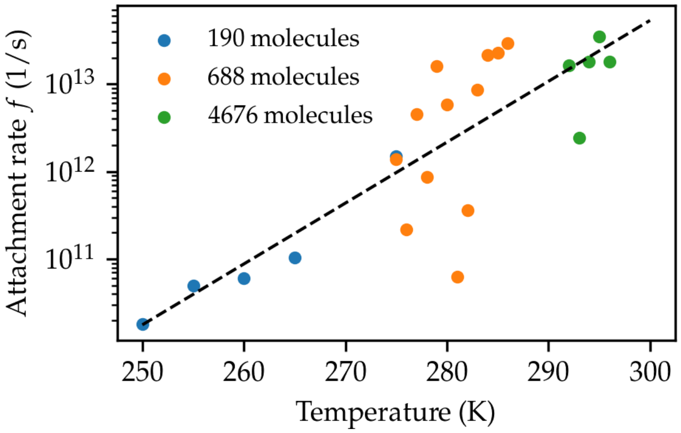


**Fig. S7. Attachment rates.** Results are shown as a function of temperature for the three cluster sizes studied in this work. An exponential fit to the data is also shown.

## 8. Driving force for nucleation and density of ice Ih

The chemical potential difference between ice Ih and liquid water $\Delta\mu_{l\to Ih}$ for different models is shown in Fig. 8a. In order to compute $\Delta\mu_{l\to Ih}$ for SCAN-ML we performed NPT simulations of liquid water and ice Ih at 1 bar and temperatures 260, 265, 270, 275, 280, 290,300, and 310 K. We computed the enthalpy difference between ice Ih and liquid water $\Delta H_{l\to Ih}$ from these simulations and obtained $\Delta\mu_{l\to Ih}$ from the thermodynamic relation,

$$\Delta\mu_{l\to Ih}(T) = T \int_{T}^{T_m^{Ih}} \frac{\Delta H_{l\to Ih}(T')}{T'^2} dT'. \qquad [6]$$

where $T_m^{Ih}$ is the melting temperature of ice Ih (310 K). The density of ice Ih for different models is shown in Fig. 8b (see Figure caption for details).

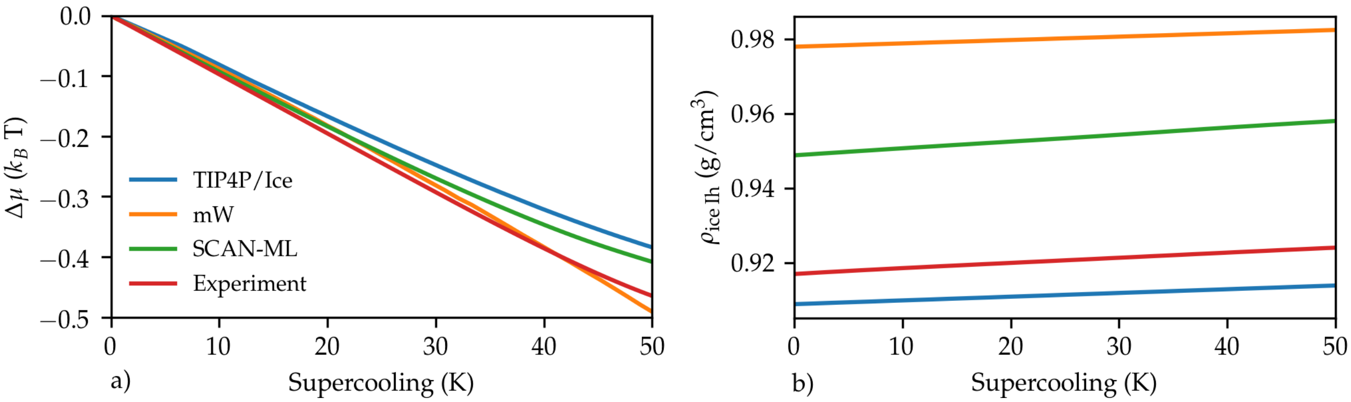


**Fig. S8. Driving force for nucleation $\Delta\mu$ and density of ice Ih.** a) Driving force for nucleation and b) density of ice Ih for the models SCAN-ML, mW, TIP4P/Ice, and from experimental measurements. $\Delta\mu$ for mW and TIP4P/Ice reproduced from Ref. 1 and the calculation of the experimental $\Delta\mu$ is described in section S12. $\rho_{\text{ice Ih}}$ for mW from Ref. 6 and for TIP4P/Ice from Ref. 7. Experimental $\rho_{\text{ice Ih}}$ calculated from data in Ref. 8.

## 9. Effect of stacking disorder on rates

In Fig. 5c we showed the effect of stacking disorder on rates using $\Delta\mu_{Ih\to Ic} = 5$ mJ/mol, i.e. a value compatible with the mW model. In Fig. S9 we show nucleation rates of ice Isd using $\Delta\mu_{Ih\to Ic} = 65$ mJ/mol, compatible with SCAN-ML. The effect of stacking disorder on rates is relatively small (around one order of magnitude) in this case.

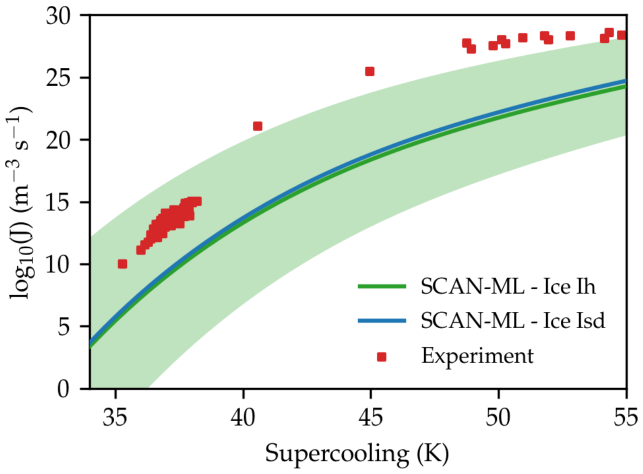


**Fig. S9. Effect of stacking disorder on rates.** The model for stacking disorder described in the main part of the article with $\Delta\mu_{Ih\to Ic} = 65$ mJ/mol was used to calculate the nucleation rate of ice Isd.

## 10. Interfacial free energy at coexistence from advanced sampling simulations

In order to calculate the interfacial free energy at coexistence we employed advanced sampling simulations. In particular, we used the On-the-fly Probability Enhanced Sampling (OPES) method(9) and a suitable collective variable (CV). The CV is based on the Environment Similarity metric(10) and for the case of ice Ih it is,

$$k_X(\chi) = \max(k_{\chi_1}(\chi), k_{\chi_2}(\chi), k_{\chi_3}(\chi), k_{\chi_4}(\chi)) \quad [7]$$

where $\chi$ is a given environment around an atom, $X = \chi_1, ..., \chi_4$ are the four reference environments of ice Ih(11), and

$$k_{\chi_k}(\chi) = \frac{1}{n} \sum_{i\in\chi} \sum_{j\in\chi_k} \exp\left(-\frac{|\mathbf{r}_i - \mathbf{r}_j^0|^2}{4\sigma^2}\right), \quad [8]$$

where $\mathbf{r}_i$ and $\mathbf{r}_j^0$ are the positions of the atoms in environments $\chi$ and $\chi_k$, respectively, $n$ is the number of atoms in the reference environment $\chi_k$, and $\sigma$ was set to 0.675 nm since this value minimizes the overlap between the distributions of $k_X$ in liquid water and ice Ih at the melting temperature. The reference environments $X$ of ice Ih are centered on each oxygen atom and included the four nearest neighbors oxygen atoms. Hydrogen atoms were not considered in the definition of the environments to allow the system to spontaneously create proton disorder. The advantage of $k_X(\chi)$ over other local order parameters that are often used for crystals is that it induces the formation of the crystal structure in a particular orientation. This feature is important to form defect free crystals.

The number of molecular environments compatible with ice Ih that exist in the whole simulation box can the be computed using,

$$n_{\text{ice Ih}} = \sum_{l=1}^{N} f(k_X(\chi^l)) \quad [9]$$

where $\chi^l$ are the $N$ environments in the simulation box, and $f(y)$ is a switching function that is zero for $k_X(\chi^l)$ values consistent with liquid water and one for $k_X(\chi^l)$ values consistent with ice Ih. $f(y)$ has to be continuous and differentiable in order to be used in advanced sampling simulations and the definition that we used in the simulations is,

$$f(y) = \begin{cases} 1 \quad \text{if} \quad y < 0 \\ (y-1)^2(1+2y) \quad \text{if} \quad 0 < y < 1 \\ 0 \quad \text{if} \quad y > 1 \end{cases}, \quad [10]$$

with $y = (k_X(\chi) - k_1)/(k_2 - k_1)$ and the values $k_1$ and $k_2$ correspond to the position of the peaks of the distributions of $k_X$ for liquid water and ice Ih, respectively.

Biasing $n_{\text{ice Ih}}$ would result in the formation of ice Ih-like environments anywhere in the simulation box and eventually lead to the crystallization of the whole simulation box. However, only the formation of a slab of ice Ih is required in order to calculate the interfacial free energy, For this reason, we also define the number of molecular environments $n_{\text{slab}}$ compatible with ice Ih that exist in a slab of width $2w$ using,

$$n_{\text{slab}} = \sum_{l=1}^{N} f(k_X(\chi^l)) g(x_l) \quad [11]$$

where $g(x_l)$ is a function that is one inside the slab and zero elsewhere, and $x_l$ is the x-component of the position of the central atom of environment $\chi_l$. The slab is centered at the x component $x_0$ of the position of oxygen atom labeled 0. In practice, we used the following definition for $g(x_l)$,

$$g(x_l) = \begin{cases} \frac{1}{\sqrt{2\pi}\epsilon} \exp\left(-\frac{(x_l - x_0)^2}{2\epsilon^2}\right) \quad \text{if} \quad |x_l - x_0| > w \\ 1 \quad \text{if} \quad |x_l - x_0| < w \end{cases}. \quad [12]$$

The width of the slab was chosen to form three crystal layers. $w$ was 0.5 nm for the basal and prismatic planes, and 0.34 nm for the secondary prismatic plane.

For the purpose of analyzing the results we defined another CV, $n_{\text{ctr}}$, based on Eq. (11). In this case the width of the slab $w'$ was chosen in order to detect the formation of the central crystalline layer of ice Ih. $w'$ was 0.14, 0.10, and 0.13 nm for the basal, prismatic, and secondary prismatic plane, respectively.

The OPES simulation was performed using $n_{\text{slab}}$ as CV and during this simulation a slab of the ice Ih crystal is reversibly formed and melted. An example of the evolution of $n_{\text{ice Ih}}$ and $n_{\text{ctr}}$ during the simulation of the basal plane is shown in Fig. S10. The bias potential became stationary after around 1 ns and this initial transient was not used for the analysis. The free energy difference between the liquid and the slab was calculated using,

$$\Delta G = -k_B T \log\left(\frac{Z^{\ddagger}}{Z^{l}}\right) \quad [13]$$

 

where $Z^{\neq}$ and $Z^{l}$ are the partition functions of the slab and the liquid. The ratio of partition functions can be conveniently written using ensemble averages,

$$\frac{Z^{\ddagger}}{Z^{l}} = \frac{\langle \delta(n_{\mathrm{layer}} - n_{\mathrm{ctr}}(\mathbf{R})) \rangle}{\langle \theta(n_{\mathrm{layer}} - n_{\mathrm{ctr}}(\mathbf{R})) \rangle} \qquad [14]$$

where $\langle \cdot \rangle$ is an ensemble average, $\delta$ is the delta function, $n_{\mathrm{layer}}$ is the number of molecules in a layer of ice Ih, and $\theta$ is the unit step function. In a biased simulation the appropriate expression is,

$$\frac{Z^{\ddagger}}{Z^{l}} = \frac{\langle e^{\beta V(\mathbf{R})} \delta(n_{\mathrm{layer}} - n_{\mathrm{ctr}}(\mathbf{R})) \rangle_V}{\langle e^{\beta V(\mathbf{R})} \theta(n_{\mathrm{layer}} - n_{\mathrm{ctr}}(\mathbf{R})) \rangle_V} \qquad [15]$$

where $V(\mathbf{R})$ is the bias potential and $\langle \cdot \rangle_V$ is an average in the biased ensemble.

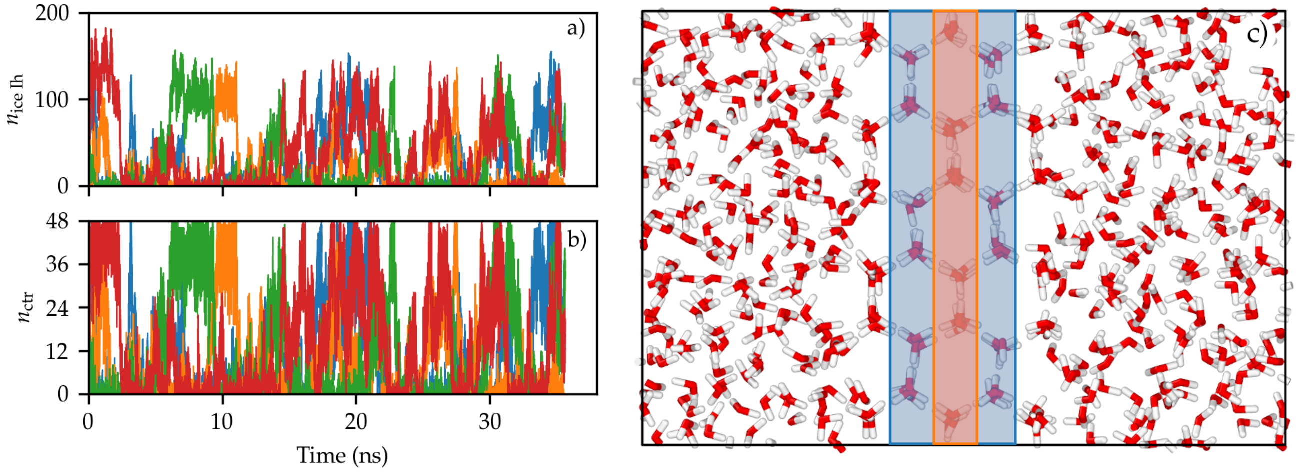


**Fig. S10. Interfacial free energy from advanced sampling simulations.** a) $n_{\mathrm{ice\ Ih}}$ vs time in a simulation of the basal plane of ice Ih exposed to the liquid. b) $n_{\mathrm{ctr}}$ vs time in a simulation of the basal plane of ice Ih exposed to the liquid. c) Planar interface between liquid water and the secondary prismatic plane of ice Ih. Regions inside which ice Ih-like molecules are counted to define $n_{\mathrm{slab}}$ (blue) and $n_{\mathrm{ctr}}$ (orange).

The free energy difference $\Delta G$ between liquid water and the slab can also be written as,

$$\Delta G = n_{\mathrm{ice\ Ih}} \Delta \mu + 2A\gamma \qquad [16]$$

where $\Delta \mu$ is the chemical potential difference between ice Ih and liquid water, $A$ the area of the cross section of the interface, and $\gamma$ is the interfacial free energy. Since by definition $\Delta \mu = 0$ at the melting temperature, $\Delta G$ includes only the contribution of the interface to the free energy. Therefore, the surface free energy can be calculated via the expression,

$$\gamma = \frac{|\Delta G|}{2A}, \qquad [17]$$

where $\Delta G$ is calculated with Eq. (13) using data from the simulation.

## 11. Interfacial free energy in $k_B T$ units

We have discussed that SCAN-ML has a melting temperature at ambient pressure of around 310 K that is somewhat higher than the experimental melting point. This feature of the model has an influence on the meaning of thermodynamic quantities that have units of energy since it changes the thermal energy $k_B T$ with respect to the experiment for a given supercooling. One way to take this effect into account for the interpretation of the interfacial free energy, is by using $k_B T$ units for the energy. In Fig. S11 we show the interfacial free energy as a function of supercooling using $k_B T$ units for the energy. In these units, the good agreement between SCAN-ML and the experiment is clearly observed.

## 12. Experimental driving force for nucleation

In order to calculate the experimental driving force for nucleation $\Delta \mu_{l \to Ih}$ based on experimental measurements, we first compute the difference in enthalpy between ice Ih and liquid water $\Delta H_{l \to Ih}$ using,

$$\Delta H_{l \to Ih}(T) = \Delta H_m + \int_{T_m^{Ih}}^{T} \left( c_p^{Ih}(T') - c_p^{l}(T') \right) dT' \qquad [18]$$

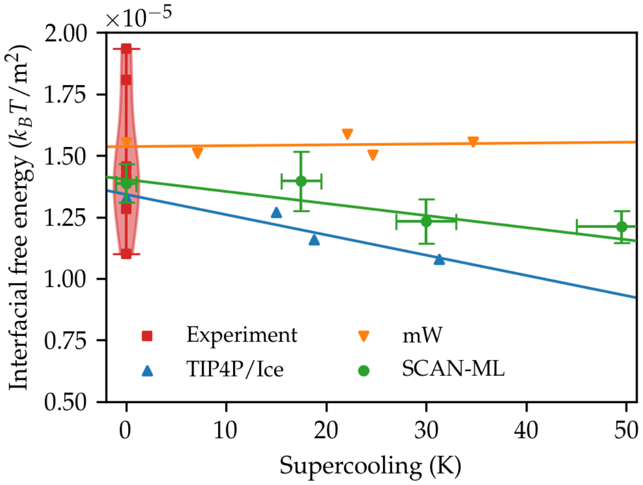


**Fig. S11. Interfacial free energy vs supercooling for the models SCAN-ML, mW, TIP4P/Ice, and from experimental measurements.** $k_B T$ is used as unit for the energy to take into account that SCAN-ML has a different melting temperature than the other models.

where $\Delta H_m = -6.01$ kJ/mol is the enthalpy of fusion, $c_p^{Ih}$ and $c_p^{l}$ are the heat capacities of ice Ih and liquid water, respectively, and $T_m^{Ih} = 273.15$ K is the melting temperature of ice Ih. We have used the heat capacity values recommended by Murphy and Koop(12). The enthalpy difference thus calculated can be used to calculate $\Delta\mu_{l\rightarrow Ih}$ employing the thermodynamic relation,

$$\Delta\mu_{l\rightarrow Ih}(T) = T \int_{T}^{T_m^{Ih}} \frac{\Delta H_{l\rightarrow Ih}(T')}{T'^2} dT'. \quad [19]$$

In this way we have calculated the reference $|\Delta\mu^{\mathrm{exp}}|$ used in Fig. 4a of the main part.

## 13. Nucleation rates with different computational techniques

In order to minimize the complexity of Figure 2, we did not specify the computational technique used to obtain the rates in the TIP4P/Ice and mW models. In Fig. S12 we show the same data as in Figure 2 using different symbols for each computational technique.

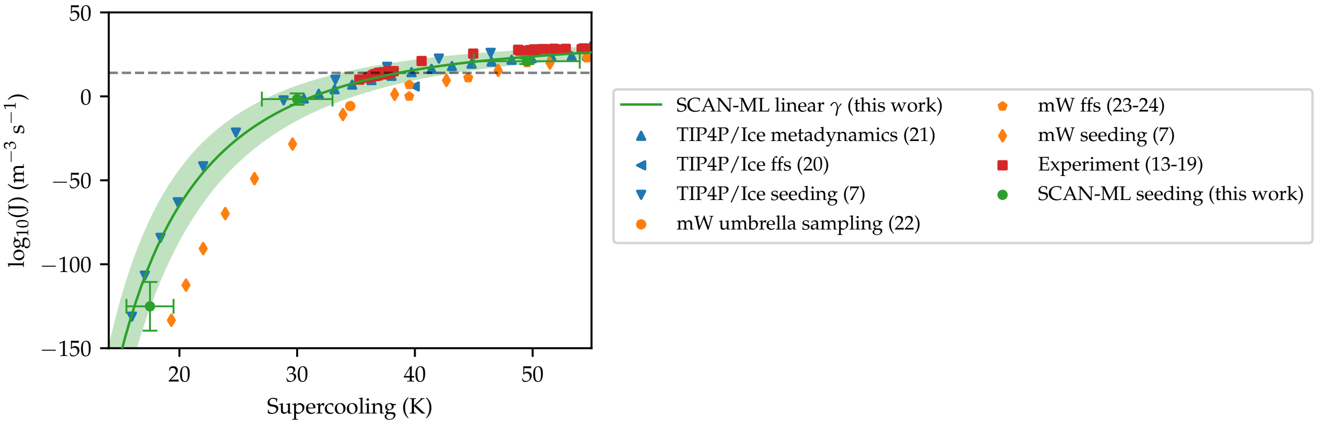


**Fig. S12. Ice nucleation rates as a function of supercooling.** Rates of the SCAN-ML model are compared with experimental data(13–19) and results from empirical models. For TIP4P/Ice we show seeding results of Espinosa et al. (7), forward flux sampling by Haji-Akbari and Debenedetti (20), and metadynamics by Niu et al. (21). For mW we show seeding results by Espinosa et al. (7), umbrella sampling calculations by Russo et al. (22), and forward flux sampling results by Li et al. (23) and Haji-Akbari et al.(24). See caption in Figure 2 for other details.

## 14. Quantum-mechanical dipole moment

We calculated the molecular dipole moment according to the modern theory of polarization(25, 26), adopting the formulation in terms of Wannier centers(27). Then, the dipole moment $\boldsymbol{\mu}_i$ of the $i$-th water molecule is given by:

$$\boldsymbol{\mu}_i = 6\, e\, \mathbf{r}_O^i + e\, \mathbf{r}_{H1}^i + e\, \mathbf{r}_{H2}^i + (-8\, e)\, \mathbf{w}_C^i \quad [20]$$

where $e$ is the elementary charge, and $\mathbf{r}_O^i$, $\mathbf{r}_{H1}^i$, $\mathbf{r}_{H2}^i$ and $\mathbf{w}_C^i$ are the positions of the oxygen atom, hydrogen atoms, and Wannier centroid of the $i$-th molecule. The charge of each oxygen atom is $+6e$ since we adopt a pseudopotential fomulation in which the atomic nuclei are replaced by ions having the charge of the nucleus minus that of the core electrons. The Wannier centroid used in Eq. (20) is defined as the geometric center of the four maximally localized Wannier functions(28) closest to each oxygen atom. The charge of the Wannier centroids is $-8e$ in Eq. (20) due to the fact that within our pseudopotential formulation there are four orbitals with two electrons each, that can be uniquely associated to each oxygen atom. The dependence of the Wannier centroids on the coordinates of the atoms in the system was described by a deep neural network (DNN) as described in ref. 29. The DNN that we use here was trained with SCAN data for liquid water and ice, as reported in ref. 30. The DeePMD-kit(31) was used to train the DNN and to calculate the position of the Wannier centroids for a given atomic configuration.

## References


1. J Espinosa, E Sanz, C Valeriani, C Vega, Homogeneous ice nucleation evaluated for several water models. *J. Chem. Phys.* **141**, 18C529 (2014).
2. BB Laird, The solid–liquid interfacial free energy of close-packed metals: Hard-spheres and the turnbull coefficient. *J. Chem. Phys.* **115**, 2887–2888 (2001).
3. D Turnbull, Formation of crystal nuclei in liquid metals. *J. Appl. Phys.* **21**, 1022–1028 (1950).
4. JR Espinosa, C Vega, E Sanz, Ice–water interfacial free energy for the tip4p, tip4p/2005, tip4p/ice, and mw models as obtained from the mold integration technique. *J. Phys. Chem. C* **120**, 8068–8075 (2016).

5. W Lechner, C Dellago, Accurate determination of crystal structures based on averaged local bond order parameters. *J. Chem. Phys.* **129**, 114707 (2008).
6. S Prestipino, The barrier to ice nucleation in monatomic water. *J. Chem. Phys.* **148**, 124505 (2018).
7. J Espinosa, C Navarro, E Sanz, C Valeriani, C Vega, On the time required to freeze water. *J. Chem. Phys.* **145**, 211922 (2016).
8. K Röttger, A Endriss, J Ihringer, S Doyle, W Kuhs, Lattice constants and thermal expansion of h2o and d2o ice ih between 10 and 265 k. *Acta Crystallogr. Sect. B: Struct. Sci.* **50**, 644–648 (1994).
9. M Invernizzi, M Parrinello, Rethinking metadynamics: from bias potentials to probability distributions. *J. Phys. Chem. Lett.* **11**, 2731–2736 (2020).
10. PM Piaggi, M Parrinello, Calculation of phase diagrams in the multithermal-multibaric ensemble. *J. Chem. Phys.* **150**, 244119 (2019).
11. PM Piaggi, R Car, Phase equilibrium of liquid water and hexagonal ice from enhanced sampling molecular dynamics simulations. *J. Chem. Phys.* **152**, 204116 (2020).
12. DM Murphy, T Koop, Review of the vapour pressures of ice and supercooled water for atmospheric applications. *Q. J. Royal Meteorol. Soc. A journal atmospheric sciences, applied meteorology physical oceanography* **131**, 1539–1565 (2005).
13. AJ Amaya, BE Wyslouzil, Ice nucleation rates near 225 k. *J. Chem. Phys.* **148**, 084501 (2018).
14. DE Hagen, RJ Anderson, JL Kassner Jr, Homogeneous condensation—freezing nucleation rate measurements for small water droplets in an expansion cloud chamber. *J. Atmos. Sci.* **38**, 1236–1243 (1981).
15. B Krämer, et al., Homogeneous nucleation rates of supercooled water measured in single levitated microdroplets. *J. Chem. Phys.* **111**, 6521–6527 (1999).
16. A Manka, et al., Freezing water in no-man's land. *Phys. Chem. Chem. Phys.* **14**, 4505–4516 (2012).
17. B Murray, et al., Kinetics of the homogeneous freezing of water. *Phys. Chem. Chem. Phys.* **12**, 10380–10387 (2010).
18. B Riechers, F Wittbracht, A Hütten, T Koop, The homogeneous ice nucleation rate of water droplets produced in a microfluidic device and the role of temperature uncertainty. *Phys. Chem. Chem. Phys.* **15**, 5873–5887 (2013).
19. CA Stan, et al., A microfluidic apparatus for the study of ice nucleation in supercooled water drops. *Lab on a Chip* **9**, 2293–2305 (2009).
20. A Haji-Akbari, PG Debenedetti, Direct calculation of ice homogeneous nucleation rate for a molecular model of water. *Proc. Natl. Acad. Sci. U. S. A.* **112**, 10582–10588 (2015).
21. H Niu, YI Yang, M Parrinello, Temperature dependence of homogeneous nucleation in ice. *Phys. Rev. Lett.* **122**, 245501 (2019).
22. J Russo, F Romano, H Tanaka, New metastable form of ice and its role in the homogeneous crystallization of water. *Nat. materials* **13**, 733–739 (2014).
23. T Li, D Donadio, G Russo, G Galli, Homogeneous ice nucleation from supercooled water. *Phys. Chem. Chem. Phys.* **13**, 19807–19813 (2011).
24. A Haji-Akbari, RS DeFever, S Sarupria, PG Debenedetti, Suppression of sub-surface freezing in free-standing thin films of a coarse-grained model of water. *Phys. Chem. Chem. Phys.* **16**, 25916–25927 (2014).
25. R Resta, Theory of the electric polarization in crystals. *Ferroelectrics* **136**, 51–55 (1992).
26. R King-Smith, D Vanderbilt, Theory of polarization of crystalline solids. *Phys. Rev. B* **47**, 1651 (1993).
27. R Resta, Macroscopic polarization in crystalline dielectrics: the geometric phase approach. *Rev. modern physics* **66**, 899 (1994).
28. N Marzari, D Vanderbilt, Maximally localized generalized wannier functions for composite energy bands. *Phys. review B* **56**, 12847 (1997).
29. L Zhang, et al., Deep neural network for the dielectric response of insulators. *Phys. Rev. B* **102**, 041121 (2020).
30. GM Sommers, MFC Andrade, L Zhang, H Wang, R Car, Raman spectrum and polarizability of liquid water from deep neural networks. *Phys. Chem. Chem. Phys.* **22**, 10592–10602 (2020).
31. H Wang, L Zhang, J Han, E Weinan, Deepmd-kit: A deep learning package for many-body potential energy representation and molecular dynamics. *Comput. Phys. Commun.* **228**, 178–184 (2018).
